# Supplementary material for: An Internal Logic of Virtual Double Categories
Source: arXiv:2410.06792 source file (2025-01-23)
Supplement: Supplementary file 1 [file eqrules.tex]

In this section, we explicitly provide
the rules for the equational theory of terms and proterms.
To begin with, we introduce some notations.
Basically, we use overlines $\ol{\bullet}$ to denote horizontal concatenation of items,
for example, $\syn{\nu}\{\ol{\syn{\mu}}/\ol{\syn{b}}\}$ means
$\syn{\nu}\{\syn{\mu}_1/\syn{b}_1:\syn{\beta}_1\smcl\dots\smcl\syn{\mu}_n/\syn{b}_n:\syn{\beta}_n\}$.
Other notations are given in \Cref{fig:abbreviations}.

    \begin{figure}[h]
    
    \begin{tabular}{|cc|c|}
    \hline
    \multicolumn{1}{|c|}{\textbf{Abbreviation}}
    & \multicolumn{1}{c|}{\textbf{Given Data}}
    & \textbf{Meaning}\\
    \hline\hline
    \multicolumn{1}{|c|}{\small$\ol{\syn{\Delta}}$}&
    \multicolumn{1}{c|}{\small$\syn{\Delta}=(\syn{\Delta}_0,\dots,\syn{\Delta}_n)$}&
    $\syn{\Delta}_0\smcl\dots\smcl\syn{\Delta}_n$
    \\
    \hline
    \multicolumn{1}{|c|}{\small$\ol{\syn{\Gamma}}=\ol{\syn{\Gamma}_{\ul{i}\,,\,\ul{j}}}$}&
    \multirow{3}{*}{
    
    \begin{tabular}{c}
    \small$\syn{\Gamma}=(\syn{\Gamma}_{i,j})_{(i,j)\in P}$\\
    \\
    {(\small The index set $P$ is the set of pairs $(i,j)$} \\{\small such that $0\leq i\leq n$ and $0\leq j\leq m_i-1$}\\
    {\small or $(i,j)=(n,m_n)$ for a given $(m_i)_{i=0}^n$.)}
    \end{tabular}}
    &
    $\syn{\Gamma}_{0,0}\smcl\syn{\Gamma}_{0,1}\smcl\dots\smcl\syn{\Gamma}_{0,n_0-1}\smcl\syn{\Gamma}_{1,0}\smcl\dots\smcl\syn{\Gamma}_{m,n_m}$
    \\
    \cline{1-1}\cline{3-3}
    \multicolumn{1}{|c|}{\small$\ol{\syn{\Gamma}_i}=\ol{\syn{\Gamma}_{i\,,\,\ul{j}}}$}&
    &
    $\syn{\Gamma}_{i,0}\smcl\syn{\Gamma}_{i,1}\smcl\dots\smcl\syn{\Gamma}_{i,n_i}$
    \\
    \cline{1-1}\cline{3-3}
    \multicolumn{1}{|c|}{\small$\wt{\syn{\Gamma}}=\wt{\syn{\Gamma}_{\ul{i}\,,\,\tilde{j}}}$}&
    &
    $\syn{\Gamma}_{0,0}\smcl\syn{\Gamma}_{1,0}\smcl\dots\smcl\syn{\Gamma}_{m,0}\smcl\syn{\Gamma}_{m,n_m}$
    \\
    \hline
    \multicolumn{1}{|c|}{\small$\ol{\syn{A}_{\ul{i}}}$}&
    \multicolumn{1}{c|}{\begin{tabular}{c}
        \small$\syn{A}_i=\syn{\alpha}_{i,0}\smcl\dots\smcl\syn{\alpha}_{i,n_i}$\quad \text{for} $1\leq i\leq m$\\
        \small$\syn{\alpha}_{i,n_i}=\syn{\alpha}_{i+1,0}$ \quad \text{for} $1\leq i\leq m-1$
        \end{tabular}}
    &
    $\syn{\alpha}_{1,0}\smcl\dots\smcl\syn{\alpha}_{1,n_1-1}\smcl\syn{\alpha}_{2,0}\smcl\dots\smcl\syn{\alpha}_{m,n_m}$
    \\
    \hline
    \end{tabular}
    \caption{Abbreviations of contexts}
    \label{fig:abbreviations}
    \end{figure}

In addition, although the presentation of replacing a variable with a term does not make sense since we follow the convention of explicit substitution,
we still use it just as an abbreviation for the sake of readability.
For example, the items on the left-hand side in the following are abbreviations for the items on the right-hand side.
    {\small
    \begin{align*}
        \syn{t}(\syn{s}_0,\dots,\syn{s}_n) &\doteq \syn{t}[\syn{s}_0/\syn{x}_0,\dots,\syn{s}_n/\syn{x}_n] \\
        \syn{\alpha}(\syn{s}_0,\dots,\syn{s}_n\smcl\syn{t}_0,\dots,\syn{t}_m) &\doteq 
        \syn{\alpha}[\syn{s}_0/\syn{x}_0,\dots,\syn{s}_n/\syn{x}_n\smcl\syn{t}_0/\syn{y}_0,\dots,\syn{t}_m/\syn{y}_m] \\
        \syn{\nu}(\overrightarrow{\syn{s}_0}\smcl\dots\smcl\overrightarrow{\syn{s}_n}) &\doteq \syn{\nu}[{\overrightarrow{\syn{s}_0}/\overrightarrow{\syn{x}_0}\smcl\dots\smcl\overrightarrow{\syn{s}_n}/\overrightarrow{\syn{x}_n}}]\\
        \syn{\nu}\{\syn{\mu}_1\smcl \dots \smcl \syn{\mu}_n\} &\doteq \syn{\nu}\{\syn{\mu}_1/\syn{b}_1,\dots,\syn{\mu}_n/\syn{b}_n\}
    \end{align*}
    }

The rules for protype isomorphisms are given as follows.
        \begin{mathparpagebreakable}
        \inferrule*
        {\syn{\Gamma} \smcl \syn{\Delta} \vdash \syn{\alpha} \ \textsf{protype}}
        {\syn{\Gamma} \smcl \syn{\Delta} \vdash \idt_{\syn{\alpha}}:\syn{\alpha}\ccong\syn{\alpha}}
        \and
        \inferrule*
        {\syn{\Gamma} \smcl \syn{\Delta} \vdash \syn{\Upsilon}:\syn{\alpha}\ccong\syn{\beta}}
        {\syn{\Gamma} \smcl \syn{\Delta} \vdash \syn{\Upsilon}^{-1}:\syn{\beta}\ccong\syn{\alpha}}
        \and
        \inferrule*
        {\syn{\Gamma} \smcl \syn{\Delta} \vdash \syn{\Upsilon}:\syn{\alpha}\ccong\syn{\beta} \\ 
        \syn{\Gamma} \smcl \syn{\Delta} \vdash \syn{\Omega}:\syn{\beta}\ccong\syn{\gamma}}
        {\syn{\Gamma} \smcl \syn{\Delta} \vdash \syn{\Omega}\circ\syn{\Upsilon}:\syn{\alpha}\ccong\syn{\gamma}}
        \and
        \inferrule*
        {\syn{\Gamma} \smcl \syn{\Delta} \vdash \syn{\alpha} \ \textsf{protype}}
        {\syn{\Gamma} \smcl \syn{\Delta} \vdash \reste: \syn{\alpha}[\syn{\Gamma}/\syn{\Gamma}\smcl\syn{\Delta}/\syn{\Delta}]
        \ccong\syn{\alpha}}
        \and
        \inferrule*
        {\syn{\Gamma}'' \vdash \syn{S}'\,/\,\syn{\Gamma}' \\ \syn{\Gamma}' \vdash \syn{S}\,/\,\syn{\Gamma} \\ 
        \syn{\Delta}'' \vdash \syn{T}'\,/\,\syn{\Delta}' \\ \syn{\Delta}' \vdash \syn{T}\,/\,\syn{\Delta} \\
        \syn{\Gamma}\smcl\syn{\Delta} \vdash \syn{\alpha} \ \textsf{protype}}
        {\syn{\Gamma}''\smcl\syn{\Delta}'' \vdash 
        \resti: \left(\syn{\alpha}[\syn{S}/\syn{\Gamma}\smcl\syn{T}/\syn{\Delta}] \right)
        [\syn{S}'/\syn{\Gamma}'\smcl\syn{T}'/\syn{\Delta}']\ccong \syn{\alpha}\left[\syn{S}[\syn{S}'/\syn{\Gamma}']/\syn{\Gamma}\smcl\syn{T}[\syn{T}'/\syn{\Delta}']/\syn{\Delta}\right] }
        \and
        \inferrule*
        {\syn{\Gamma}' \vdash \syn{S}\,/\,\syn{\Gamma} \\ \syn{\Delta}' \vdash \syn{T}\,/\,\syn{\Delta} \\ 
        \syn{\Gamma}\smcl\syn{\Delta} \vdash \syn{\alpha} \ \textsf{protype}\\ \syn{\Gamma}\smcl\syn{\Delta} \vdash \syn{\beta} \ \textsf{protype}}
        {\syn{\Gamma}'\smcl\syn{\Delta}' \vdash
        \rest_{\land}:\left(\syn{\alpha}\land\syn{\beta}\right)[\syn{S}/\syn{\Gamma}\smcl\syn{T}/\syn{\Delta}] \ccong \syn{\alpha}[\syn{S}/\syn{\Gamma}\smcl\syn{T}/\syn{\Delta}]\land\syn{\beta}[\syn{S}/\syn{\Gamma}\smcl\syn{T}/\syn{\Delta}]}
        \and
        \inferrule*
        {\syn{\Gamma}' \vdash \syn{S}\,/\,\syn{\Gamma} \\ \syn{\Delta}' \vdash \syn{T}\,/\,\syn{\Delta}}
        {\syn{\Gamma}'\smcl\syn{\Delta}' \vdash
        \rest_{\top}:\top[\syn{S}/\syn{\Gamma}\smcl\syn{T}/\syn{\Delta}] \ccong \top}
        \and
        \inferrule*
        {\syn{\Gamma}' \vdash \syn{S}_0\,/\,\syn{\Gamma}\equiv \syn{S}_1\,/\,\syn{\Gamma}\\
        \syn{\Delta}' \vdash \syn{T}_0\,/\,\syn{\Delta}\equiv \syn{T}_1\,/\,\syn{\Delta}\\
        \syn{\Gamma}'\smcl\syn{\Delta}' \vdash \syn{\alpha} \ \textsf{protype} }
        {\syn{\Gamma}'\smcl\syn{\Delta}' \vdash 
        \repl_{\syn{S}_0,\syn{S}_1\smcl\syn{T}_0,\syn{T}_1}:\syn{\alpha}[\syn{S}_0/\syn{\Gamma}\smcl\syn{T}_0/\syn{\Delta}] \ccong
        \syn{\alpha}[\syn{S}_1/\syn{\Gamma}\smcl\syn{T}_1/\syn{\Delta}]}
        \and 
        \inferrule*
        {\syn{\Gamma}\smcl\syn{\Delta} \mid \syn{a}:\syn{\alpha} \vdash \syn{\mu}\{\syn{a}\}:\syn{\beta} \\
        \syn{\Gamma}\smcl\syn{\Delta} \mid \syn{b}:\syn{\beta} \vdash \syn{\nu}\{\syn{b}\}:\syn{\alpha}\\
        \syn{\Gamma}\smcl\syn{\Delta} \mid \syn{b}:\syn{\beta} \vdash \syn{\mu}\{\syn{\nu}\{\syn{b}\}\}\equiv \syn{b}:\syn{\beta}\\
        \syn{\Gamma}\smcl\syn{\Delta} \mid \syn{a}:\syn{\alpha} \vdash \syn{\nu}\{\syn{\mu}\{\syn{a}\}\}\equiv \syn{a}:\syn{\alpha}}
        {\syn{\Gamma}\smcl\syn{\Delta} \vdash \lcp\syn{\mu},\syn{\nu}\rcp:\syn{\alpha}\ccong\syn{\beta}}         
        \and
        \inferrule*
        {\syn{\Gamma}\smcl\syn{\Delta} \mid \syn{a}:\syn{\alpha} \vdash \syn{\mu}\{\syn{a}\}:\syn{\beta} \\
        \syn{\Gamma}\smcl\syn{\Delta} \mid \syn{b}:\syn{\beta} \vdash \syn{\nu}\{\syn{b}\}:\syn{\alpha}\\
        \syn{\Gamma}\smcl\syn{\Delta} \mid \syn{b}:\syn{\beta} \vdash \syn{\mu}\{\syn{\nu}\{\syn{b}\}\}\equiv \syn{b}:\syn{\beta}\\
        \syn{\Gamma}\smcl\syn{\Delta} \mid \syn{a}:\syn{\alpha} \vdash \syn{\nu}\{\syn{\mu}\{\syn{a}\}\}\equiv \syn{a}:\syn{\alpha}}
        {\syn{\Gamma}\smcl\syn{\Delta} \mid \syn{a}:\syn{\alpha} \vdash \lcp\syn{\mu},\syn{\nu}\rcp\{\syn{a}\}\equiv \syn{\mu}\{\syn{a}\}:\syn{\beta}}
    \end{mathparpagebreakable}

The rules for the equational theory of proterms are given as follows.
It is worth noting that there are some rules for the conversion $\trr_{\syn{\Upsilon}}\{\syn{a}\}$
to guarantee that the introduced protype isomorphisms behave as expected.  
For example, we have the rule $\lcp\syn{\mu},\syn{\nu}\rcp\{\syn{a}\}\equiv\syn{\mu}\{\syn{a}\}$
for the proterm $\syn{\mu}$ and $\syn{\nu}$ that are mutually inverse to each other,
and the rule $\syn{\Upsilon}\inv\{\syn{\Upsilon}\{\syn{a}\}\}\equiv\syn{a}$ for a protype isomorphism $\syn{\Upsilon}$.
From these rules, one can derive that the inverse of $\lcp\syn{\mu},\syn{\nu}\rcp$ also has the expected behavior: 
    $
        \lcp\syn{\mu},\syn{\nu}\rcp\inv\{\syn{b}\} 
        \equiv \lcp\syn{\nu},\syn{\mu}\rcp\inv\left\{\syn{\mu}\left\{\syn{\nu}\{\syn{b}\}\right\}\right\}
        \equiv \lcp\syn{\nu},\syn{\mu}\rcp\inv\left\{\lcp\syn{\nu},\syn{\mu}\rcp\left\{\syn{\nu}\{\syn{b}\}\right\}\right\}
        \equiv \syn{\nu}\{\syn{b}\}
    $.

\paragraph*{Equational theory of proterms}\
        \begin{mathparpagebreakable}
        \goodbreak
        \inferrule*
        {\syn{\Gamma}_0\smcl\dots\smcl\syn{\Gamma}_n\mid
        \syn{a}_1:\syn{\alpha}_1\smcl\dots\smcl\syn{a}_n:\syn{\alpha}_n\vdash \syn{\mu}:\syn{\beta} }
        {\syn{\Gamma}_0\smcl\dots\smcl\syn{\Gamma}_n\mid\syn{a}_1:\syn{\alpha}_1\smcl\dots\smcl\syn{a}_n:\syn{\alpha}_n\vdash 
        \syn{b}\{\syn{\mu}\}\equiv \syn{\mu}:\syn{\beta}}
        \and
        \inferrule*
        {\syn{\Gamma}_0\smcl\dots\smcl\syn{\Gamma}_n\mid
        \syn{a}_1:\syn{\alpha}_1\smcl\dots\smcl\syn{a}_n:\syn{\alpha}_n\vdash \syn{\mu}:\syn{\beta} }
        {\syn{\Gamma}_0\smcl\dots\smcl\syn{\Gamma}_n\mid\syn{a}_1:\syn{\alpha}_1\smcl\dots\smcl\syn{a}_n:\syn{\alpha}_n\vdash
        \syn{\mu}\{\syn{a}_1\smcl\dots\smcl\syn{a}_n\}\equiv
        \syn{\mu}:\syn{\beta}}
        \and
        \inferrule*
        {\ol{\syn{\Gamma}}\mid \syn{A}\vdash \syn{\mu}:\syn{\alpha}\\
        \ol{\syn{\Gamma}}\mid \syn{A}\vdash \syn{\nu}:\syn{\beta}}
        {\ol{\syn{\Gamma}}\mid \syn{A}\vdash \syn{\pi}_0\{\langle \syn{\mu},\syn{\nu} \rangle\}\equiv \syn{\mu}:\syn{\alpha}}
        \and
        \inferrule*
        {\ol{\syn{\Gamma}}\mid \syn{A}\vdash \syn{\mu}:\syn{\alpha}\\
        \ol{\syn{\Gamma}}\mid \syn{A}\vdash \syn{\nu}:\syn{\beta}}
        {\ol{\syn{\Gamma}}\mid \syn{A}\vdash \syn{\pi}_1\{\langle \syn{\mu},\syn{\nu} \rangle\}\equiv \syn{\nu}:\syn{\beta}}
        \and
        \inferrule*
        {\ol{\syn{\Gamma}}\mid \syn{A}\vdash \syn{\mu}:\syn{\alpha}\land\syn{\beta}}
        {\ol{\syn{\Gamma}}\mid \syn{A}\vdash \langle \syn{\pi}_0\{\syn{\mu}\},\syn{\pi}_1\{\syn{\mu}\}\rangle\equiv \syn{\mu}:\syn{\alpha}\land\syn{\beta}}
        \and 
        \inferrule*
        {\ol{\syn{\Gamma}}\mid \syn{A}\vdash \syn{\mu}:\top}
        {\ol{\syn{\Gamma}}\mid \syn{A}\vdash \syn{\mu}\equiv \langle \ \rangle:\top}
        \and
        \inferrule*
        {\ol{\syn{\Gamma}_i}\mid \syn{A}_i\vdash \syn{\mu}_i:\syn{\beta}_i \quad (i=1,\dots,n)\\
        \wt{\syn{\Gamma}}\mid \syn{\beta}_1,\dots,\syn{\beta}_n\vdash \syn{\nu}_j:\syn{\gamma}_j \quad (j=1,2)}
        {\ol{\syn{\Gamma}}\mid \ol{\syn{A}_{\ul{i}}}\vdash \langle \syn{\nu}_1,\syn{\nu}_2 \rangle\{\ol{\syn{\mu}}/\ol{\syn{b}}\}\equiv
        \langle \syn{\nu}_1\{\ol{\syn{\mu}}/\ol{\syn{b}}\},\syn{\nu}_2\{\ol{\syn{\mu}}/\ol{\syn{b}}\} \rangle:\syn{\gamma}_1\land\syn{\gamma}_2}
        \and
        \inferrule*
        {\ol{\syn{\Gamma}_i}\mid \syn{A}_i\vdash \syn{\mu}_i:\syn{\beta}_i \quad (i=1,\dots,n)\\
        \wt{\syn{\Gamma}}\mid \syn{\beta}_1,\dots,\syn{\beta}_n\vdash \syn{\nu}:\syn{\gamma_1}\land\syn{\gamma_2}}
        {\ol{\syn{\Gamma}}\mid \ol{\syn{A}_{\ul{i}}}\vdash \syn{\pi}_0\{\syn{\nu}\{\ol{\syn{\mu}}/\ol{\syn{b}}\}\}\equiv
        \syn{\pi}_0\{\syn{\nu}\}\{\ol{\syn{\mu}}/\ol{\syn{b}}\}:\syn{\gamma}_1}
        \and
        \inferrule*
        {\ol{\syn{\Gamma}_i}\mid \syn{A}_i\vdash \syn{\mu}_i:\syn{\beta}_i \quad (i=1,\dots,n)\\
        \wt{\syn{\Gamma}}\mid \syn{\beta}_1,\dots,\syn{\beta}_n\vdash \syn{\nu}:\syn{\gamma_1}\land\syn{\gamma_2}}
        {\ol{\syn{\Gamma}}\mid \ol{\syn{A}_{\ul{i}}}\vdash \syn{\pi}_1\{\syn{\nu}\{\ol{\syn{\mu}}/\ol{\syn{b}}\}\}\equiv
        \syn{\pi}_1\{\syn{\nu}\}\{\ol{\syn{\mu}}/\ol{\syn{b}}\}:\syn{\gamma}_2}
        \and
        \inferrule*
        {\ol{\syn{\Gamma}_{i,j,\ul{k}}}\mid \syn{A}_{i,j}\vdash \syn{\mu}_{i,j}:\syn{\beta}_{i,j} \quad (i=1,\dots,m,\ j=1,\dots,n_i)\\    
        \wt{\syn{\Gamma}_{i,\ul{j},\wt{k}}}\mid \syn{b}_{i,1}:\syn{\beta}_{i,1}\smcl\dots\syn{b}_{i,n_i}:\syn{\beta}_{i,n_i}\vdash \syn{\nu}_i:\syn{\gamma}_i \quad (i=1,\dots,m)\\
        \wt{\syn{\Gamma}_{\ul{i},\wt{j},\wt{k}}}\mid \syn{c}_1:\syn{\gamma}_1\smcl\dots\smcl\syn{c}_m:\syn{\gamma}_m\vdash \syn{\lambda}:\syn{\delta}}
        {\ol{\syn{\Gamma}}\mid\ol{\syn{A}}\vdash 
        \left(\syn{\lambda}\{\ol{\syn{\nu}}/\ol{\syn{c}}\}\right)
        \{\ol{\syn{\mu}}/\ol{\syn{b}}:\ol{\syn{\beta}}\}\equiv
        \syn{\lambda}\left\{\left.\ol{\syn{\nu}_{\ul{i}}\{\ol{\syn{\mu}_{i,\ul{j}}}/\ol{\syn{b}_{i,\ul{j}}}}\}\right/
        \ol{\syn{c}}\right\}:\syn{\delta}}
        \and
        \inferrule*
        {\syn{\Gamma}_i\vdash\syn{S}_i\,/\,\syn{\Delta}_i \ (i=1,\dots,n) \\ 
        \ol{\syn{\Delta}}\mid \syn{A}\vdash \syn{\mu}:\syn{\beta}\\
        \ol{\syn{\Delta}}\mid \syn{A}\vdash \syn{\nu}:\syn{\gamma}}
        {\ol{\syn{\Gamma}}\mid \syn{A}[\ol{\syn{S}}/\ol{\syn{\Delta}}]\vdash
        \langle\syn{\mu},\syn{\nu}\rangle[\syn{S}_0/\syn{\Delta}_0\smcl\dots\smcl\syn{S}_n/\syn{\Delta}_n]\equiv
        \left\langle \syn{\mu}[\ol{\syn{S}}/\ol{\syn{\Delta}}],\syn{\nu}[\ol{\syn{S}}/\ol{\syn{\Delta}}]\right\rangle:
        \left(\syn{\beta}\land\syn{\gamma}\right)[\syn{S}_0/\syn{\Delta}_0\smcl\syn{S}_n/\syn{\Delta}_n]}
        \and
        \inferrule*
        {\syn{\Gamma}_i\vdash\syn{S}_i\,/\,\syn{\Delta}_i\ (i=1,\dots,n)\\
        \ol{\syn{\Delta}}\mid \syn{A}\vdash \syn{\mu}:\syn{\beta}\land\syn{\gamma}}
        {\ol{\syn{\Gamma}}\mid \syn{A}[\ol{\syn{S}}/\ol{\syn{\Delta}}]\vdash
        \syn{\pi}_0\{\syn{\mu}[\ol{\syn{S}}/\ol{\syn{\Delta}}]\}\equiv
        \syn{\pi}_0\{\syn{\mu}\}[\ol{\syn{S}}/\ol{\syn{\Delta}}]:
        \syn{\beta}[\syn{S}_0/\syn{\Delta}_0\smcl\syn{S}_n/\syn{\Delta}_n]}
        \and
        \inferrule*
        {\syn{\Gamma}_i\vdash\syn{S}_i\,/\,\syn{\Delta}_i \ (i=1,\dots,n)\\
        \ol{\syn{\Delta}}\mid \syn{A}\vdash \syn{\mu}:\syn{\beta}\land\syn{\gamma}}
        {\ol{\syn{\Gamma}}\mid \syn{A}[\ol{\syn{S}}/\ol{\syn{\Delta}}]\vdash
        \syn{\pi}_1\{\syn{\mu}[\ol{\syn{S}}/\ol{\syn{\Delta}}]\}\equiv
        \syn{\pi}_1\{\syn{\mu}\}[\ol{\syn{S}}/\ol{\syn{\Delta}}]:
        \syn{\gamma}[\syn{S}_0/\syn{\Delta}_0\smcl\syn{S}_n/\syn{\Delta}_n]}
        \and
        \inferrule*
        {\syn{\Gamma}_i\vdash\syn{S}_i\,/\,\syn{\Delta}_i \ (i=1,\dots,n)\\
        \syn{\Delta}_i\vdash\syn{T}_i\,/\,\syn{\Theta}_i \ (i=1,\dots,n)\\
        \ol{\syn{\Theta}}\mid \syn{A}\vdash \syn{\mu}:\syn{\beta}}
        {\ol{\syn{\Gamma}}\mid \syn{A}[\ol{\syn{T}}/\ol{\syn{\Theta}}][\ol{\syn{S}}/\ol{\syn{\Delta}}]
        \vdash\left(\syn{\mu}[\ol{\syn{T}}/\ol{\syn{\Theta}}]\right)[\ol{\syn{S}}/\ol{\syn{\Delta}}]\equiv
        \syn{\mu}\left[\ol{\syn{T}}[\ol{\syn{S}}/\ol{\syn{\Delta}}]/\ol{\syn{\Theta}}\right]:
        \syn{\beta}[\syn{T}_0/\syn{\Theta}_0\smcl\syn{T}_n/\syn{\Theta}_n][\syn{S}_0/\syn{\Delta}_0\smcl\syn{S}_n/\syn{\Delta}_n]}
        \and
        \inferrule*
        {\syn{\Gamma}_{i,j}\vdash\syn{S}_{i,j}\,/\,\syn{\Delta}_{i,j} \ (i=1,\dots,m,\ j=1,\dots,n_i)\\
        \ol{\syn{\Delta}_{i,\ul{j}}}\mid \syn{A}_i \vdash \syn{\mu}_i:\syn{\beta}_i \ (i=1,\dots,m) \\
        \wt{\syn{\Delta}_{\ul{i},\tilde{j}}} \mid\syn{b}_1:\syn{\beta}_1\smcl\dots\smcl\syn{b}_n:\syn{\beta}_n \vdash\syn{\nu}: \syn{\gamma}}
        {\syn{\ol{\Gamma}}\mid \ol{\syn{A}}[\ol{\syn{S}}/\ol{\syn{\Delta}}]\vdash
        \syn{\nu}\{\ol{\syn{\mu}}/\ol{\syn{b}}\}[\ol{\syn{S}}/\ol{\syn{\Delta}}]\equiv
        \syn{\nu}\left[\left.\wt{\syn{S}_{\ul{i},\tilde{j}}}\right/\wt{\syn{\Delta}_{\ul{i},\tilde{j}}}\right]
        \left\{\left.\ol{\syn{\mu}_{\ul{i}}[\ol{\syn{S}_{i,\ul{j}}}/\ol{\syn{\Delta}_{i,\ul{j}}}]}\right/
        \ol{\syn{b}_{\ul{i}}}\right\}:
        \syn{\gamma}[\syn{S}_{0,0}/\syn{\Delta}_{0,0}\smcl\syn{S}_{m,n_m}/\syn{\Delta}_{m,n_m}]}
        \and
        \inferrule*
        {\syn{\Gamma}\smcl\syn{\Delta}\vdash \syn{\alpha} \ \textsf{protype}}
        {\syn{\Gamma}\smcl\syn{\Delta}\mid \syn{a}:\syn{\alpha}\vdash \idt_{\syn{\alpha}}\{\syn{a}\}\equiv \syn{a}:\syn{\alpha}}
        \and
        \inferrule*
        {\syn{\Gamma}\smcl\syn{\Delta}\vdash \syn{\Upsilon}:\syn{\alpha}\ccong\syn{\beta}}
        {\syn{\Gamma}\smcl\syn{\Delta}\mid \syn{a}:\syn{\alpha}\vdash \syn{\Upsilon}^{-1}\{\syn{\Upsilon}\{\syn{a}\}\}\equiv \syn{a}:\syn{\alpha}}
        \and  
        \inferrule*
        {\syn{\Gamma}\smcl\syn{\Delta}\vdash \syn{\Upsilon}:\syn{\alpha}\ccong\syn{\beta}}
        {\syn{\Gamma}\smcl\syn{\Delta}\mid \syn{b}:\syn{\beta} \vdash \syn{\Upsilon}\{\syn{\Upsilon}^{-1}\{\syn{a}\}\}\equiv \syn{a}:\syn{\alpha}}
        \and
        \inferrule*
        {\syn{\Gamma}\smcl\syn{\Delta}\vdash \syn{\Upsilon}:\syn{\alpha}\ccong\syn{\beta}\\
        \syn{\Gamma}\smcl\syn{\Delta}\vdash \syn{\Omega}:\syn{\beta}\ccong\syn{\gamma}}
        {\syn{\Gamma}\smcl\syn{\Delta}\mid \syn{a}:\syn{\alpha}\vdash (\syn{\Omega}\circ\syn{\Upsilon})\{\syn{a}\}\equiv
        \syn{\Omega}\{\syn{\Upsilon}\{\syn{a}\}\}:\syn{\gamma}}
        \and  
        \inferrule*
        {\syn{\Gamma}\smcl\syn{\Delta}\vdash \syn{\alpha} \ \textsf{protype}\\
        \syn{\Gamma}'\vdash \syn{S}\,/\,\syn{\Gamma} \\ \syn{\Delta}'\vdash \syn{T}\,/\,\syn{\Delta}}
        {\syn{\Gamma}'\smcl\syn{\Delta'}\mid \syn{a}:\syn{\alpha}[\syn{S}/\syn{\Gamma}\smcl\syn{T}/\syn{\Delta}]\vdash
        \repl_{\syn{S},\syn{S}\smcl\syn{T},\syn{T}}\{\syn{a}\}\equiv \syn{a}:\syn{\alpha}[\syn{S}/\syn{\Gamma}\smcl\syn{T}/\syn{\Delta}]}
        \and   
        \inferrule*
        {\syn{\Gamma}' \vdash \syn{S}_0\,/\,\syn{\Gamma}\equiv \syn{S}_1\,/\,\syn{\Gamma}\\
        \syn{\Delta}' \vdash \syn{T}_0\,/\,\syn{\Delta}\equiv \syn{T}_1\,/\,\syn{\Delta}\\
        \syn{\Gamma}'\smcl\syn{\Delta}' \vdash \syn{\alpha} \ \textsf{protype} }
        {\syn{\Gamma}'\smcl\syn{\Delta}'\mid \syn{a}:\syn{\alpha}\left[\syn{S}_0/\syn{\Gamma}\smcl\syn{T}_0/\syn{\Delta}\right]\vdash
        \repl_{\syn{S}_0,\syn{S}_1\smcl\syn{T}_0,\syn{T}_1}\{\syn{a}\}\equiv 
        \repl_{\syn{S}_1,\syn{S}_0\smcl\syn{T}_1,\syn{T}_0}\inv\{\syn{a}\}:\syn{\alpha}\left[\syn{S}_1/\syn{\Gamma}\smcl\syn{T}_1/\syn{\Delta}\right]}
        \and 
        \inferrule*
        {\syn{\Gamma}' \vdash \syn{S}_0\,/\,\syn{\Gamma}\equiv \syn{S}_1\,/\,\syn{\Gamma}\\
        \syn{\Gamma}' \vdash \syn{S}_1\,/\,\syn{\Gamma}\equiv \syn{S}_2\,/\,\syn{\Gamma}\\
        \syn{\Delta}' \vdash \syn{T}_0\,/\,\syn{\Delta}\equiv \syn{T}_1\,/\,\syn{\Delta}\\
        \syn{\Delta}' \vdash \syn{T}_1\,/\,\syn{\Delta}\equiv \syn{T}_2\,/\,\syn{\Delta}\\
        \syn{\Gamma}'\smcl\syn{\Delta}' \vdash \syn{\alpha} \ \textsf{protype} }
        {\syn{\Gamma}'\smcl\syn{\Delta}'\mid \syn{a}:\syn{\alpha}\left[\syn{S}_0/\syn{\Gamma}\smcl\syn{T}_0/\syn{\Delta}\right]\vdash
        \repl_{\syn{S}_1,\syn{S}_2\smcl\syn{T}_1,\syn{T}_2}\{\repl_{\syn{S}_0,\syn{S}_1\smcl\syn{T}_0,\syn{T}_1}\{\syn{a}\}\}\equiv
        \repl_{\syn{S}_0,\syn{S}_2\smcl\syn{T}_0,\syn{T}_2}\{\syn{a}\}:\syn{\alpha}\left[\syn{S}_2/\syn{\Gamma}\smcl\syn{T}_2/\syn{\Delta}\right]}
        \and 
        \inferrule*
        {\syn{\Gamma'}\vdash \syn{S}\,/\,\syn{\Gamma} \\ \syn{\Delta'}\vdash \syn{T}\,/\,\syn{\Delta} \\
        \syn{\Gamma}\smcl\syn{\Delta}\vdash \syn{\alpha} \ \textsf{protype}\\
        \syn{\Gamma}\smcl\syn{\Delta}\vdash \syn{\beta} \ \textsf{protype}}
        {\syn{\Gamma'}\smcl\syn{\Delta'}\mid \syn{a}:(\syn{\alpha}\land\syn{\beta})[\syn{S}/\syn{\Gamma}\smcl\syn{T}/\syn{\Delta}]\vdash
        \rest_{\land}\{\syn{a}\}\equiv \left\langle \syn{\pi}_0[\syn{S}/\syn{\Gamma}\smcl\syn{T}/\syn{\Delta}],
        \syn{\pi}_1[\syn{S}/\syn{\Gamma}\smcl\syn{T}/\syn{\Delta}]\right\rangle:\syn{\alpha}[\syn{S}/\syn{\Gamma}\smcl\syn{T}/\syn{\Delta}]\land\syn{\beta}[\syn{S}/\syn{\Gamma}\smcl\syn{T}/\syn{\Delta}]} 
        \and
        \inferrule*
        {\syn{\Gamma}\smcl\syn{\Delta} \mid \syn{a}:\syn{\alpha} \vdash \syn{\mu}\{\syn{a}\}:\syn{\beta} \\
        \syn{\Gamma}\smcl\syn{\Delta} \mid \syn{b}:\syn{\beta} \vdash \syn{\nu}\{\syn{b}\}:\syn{\alpha}\\
        \syn{\Gamma}\smcl\syn{\Delta} \mid \syn{b}:\syn{\beta} \vdash \syn{\mu}\{\syn{\nu}\{\syn{b}\}\}\equiv \syn{b}:\syn{\beta}\\
        \syn{\Gamma}\smcl\syn{\Delta} \mid \syn{a}:\syn{\alpha} \vdash \syn{\nu}\{\syn{\mu}\{\syn{a}\}\}\equiv \syn{a}:\syn{\alpha}}
        {\syn{\Gamma}\smcl\syn{\Delta} \mid \syn{a}:\syn{\alpha} \vdash \lcp\syn{\mu},\syn{\nu}\rcp\{\syn{a}\}\equiv \syn{\mu}\{\syn{a}\}:\syn{\beta}}
        \and  
        \inferrule*
        {\syn{\Gamma} \smcl \syn{\Delta} \vdash \syn{\alpha} \ \textsf{protype}\\
        \syn{\Gamma}'\vdash \syn{S}\,/\,\syn{\Gamma} \\ \syn{\Delta}'\vdash \syn{T}\,/\,\syn{\Delta}}
        {\syn{\Gamma}'\smcl\syn{\Delta'}\mid \syn{a}:\syn{\alpha}[\syn{\Gamma}/\syn{\Gamma}\smcl\syn{\Delta}/\syn{\Delta}][\syn{S}/\syn{\Gamma}\smcl\syn{T}/\syn{\Delta}]\vdash
        \reste\{\syn{a}\}[\syn{S}/\syn{\Gamma}\smcl\syn{T}/\syn{\Delta}]\equiv 
        \resti\{\syn{a}\}:\syn{\alpha}[\syn{S}/\syn{\Gamma}\smcl\syn{T}/\syn{\Delta}]} 
        \and
        \inferrule*
        {\syn{\Gamma} \smcl \syn{\Delta} \vdash \syn{\alpha} \ \textsf{protype}\\
        \syn{\Gamma}'\vdash \syn{S}\,/\,\syn{\Gamma} \\ \syn{\Delta}'\vdash \syn{T}\,/\,\syn{\Delta}}
        {
        \syn{\Gamma}'\smcl\syn{\Delta'}\mid \syn{a}:\syn{\alpha}[\syn{S}/\syn{\Gamma}\smcl\syn{T}/\syn{\Delta}][\syn{\Gamma}/\syn{\Gamma}\smcl\syn{\Delta}/\syn{\Delta}]\vdash
        \reste\{\syn{a}\}\equiv \resti\{\syn{a}\}:\syn{\alpha}[\syn{S}/\syn{\Gamma}\smcl\syn{T}/\syn{\Delta}]} 
        \and
        \inferrule*
        {{\syn{\Gamma}_{i+1}}\vdash \syn{S}_{i}\,/\,\syn{\Gamma}_{i} \ (i=0,1,2)\\
        \syn{\Delta}_{i+1}\vdash \syn{T}_{i}\,/\,\syn{\Delta}_{i} \ (i=0,1,2)\\
        \syn{\Gamma}_0\smcl\syn{\Delta}_0 \vdash \syn{\alpha} \ \textsf{protype}}
        {
        {\begin{array}{l}    
        \syn{\Gamma}_3\smcl\syn{\Delta}_3\mid \syn{a}: \syn{\alpha}[{\syn{S}_0/\syn{\Gamma}_0}\smcl{\syn{T}_0/\syn{\Delta}_0}]
        [{\syn{S}_1/\syn{\Gamma}_1}\smcl{\syn{T}_1/\syn{\Delta}_1}][{\syn{S}_1/\syn{\Gamma}_2}\smcl{\syn{T}_2/\syn{\Delta}_2}]\\
        \qquad\vdash
        \resti\left\{\resti\{\syn{a}\}[\syn{S}_2/\syn{\Gamma}_2\smcl\syn{T}_2/\syn{\Delta}_2]\right\}
        \equiv 
        \resti\left\{\resti\{\syn{a}\}\right\}:\syn{\alpha}
        \left[\left.
        \syn{S}_0[{\syn{S}_1/\syn{\Gamma}_1}][{\syn{S}_2/\syn{\Gamma}_2}]\right/\syn{\Gamma}_0\smcl
        \left.
        \syn{T}_0[{\syn{T}_1/\syn{\Delta}_1}][{\syn{T}_2/\syn{\Delta}_2}]\right/\syn{\Delta}_0\right]
        \end{array}}
        }
        \and
        \inferrule*
        {{\syn{\Gamma}_{i+1}}\vdash \syn{S}_{i}\,/\,\syn{\Gamma}_{i} \ (i=0,1)\\
        \syn{\Delta}_{i+1}\vdash \syn{T}_{i}\,/\,\syn{\Delta}_{i} \ (i=0,1)\\
        \syn{\Gamma}_0\smcl\syn{\Delta}_0 \vdash \syn{\alpha} \ \textsf{protype}\\
        \syn{\Gamma}_0\smcl\syn{\Delta}_0 \vdash \syn{\beta} \ \textsf{protype}}
        {
        {\begin{array}{l}
        \syn{\Gamma}_2\smcl\syn{\Delta}_2\mid \syn{a}:\left(\syn{\alpha}\land\syn{\beta}\right)
        [{\syn{S}_0/\syn{\Gamma}_0}\smcl{\syn{T}_0/\syn{\Delta}_0}]
        [{\syn{S}_1/\syn{\Gamma}_1}\smcl{\syn{T}_1/\syn{\Delta}_1}]
        \\
        \qquad\vdash
        \rest_{\land}\left\{\resti\{\syn{a}\}\right\}
        \equiv
        \left\langle \resti\{\syn{\pi}_0\{\syn{a}\}\},\resti\{\syn{\pi}_1\{\syn{a}\}\}\right\rangle
        \left\{\rest_{\land}\left\{\rest_{\land}\{\syn{a}\}[{\syn{S}_1/\syn{\Gamma}_1}\smcl{\syn{T}_1/\syn{\Delta}_1}]\right\}/\syn{a}\right\}
        \\
        \qquad:\syn{\alpha}\left[\left.
            \syn{S}_0[{\syn{S}_1/\syn{\Gamma}_1}]\right/\syn{\Gamma}_0\smcl
            \left.
            \syn{T}_0[{\syn{T}_1/\syn{\Delta}_1}]\right/\syn{\Delta}_0\right]
        \land\syn{\beta}\left[\left.
            \syn{S}_1\right/\syn{\Gamma}_1\smcl
            \left.
            \syn{T}_1\right/\syn{\Delta}_1\right]
        \end{array}}
        }
        \and             
        \inferrule*
        {{\syn{\Gamma}_1}\vdash \syn{S}_0/\syn{\Gamma}_0 \equiv \syn{S}_0'/\syn{\Gamma}_0\\
        {\syn{\Delta}_1}\vdash \syn{T}_0/\syn{\Delta}_0 \equiv \syn{T}_0'/\syn{\Delta}_0\\ 
        \syn{\Gamma}_2\vdash \syn{S}_1\,/\,\syn{\Gamma}_1 \\
        \syn{\Delta}_2\vdash \syn{T}_1\,/\,\syn{\Delta}_1 \\
        }
        {
        {\begin{array}{l}
        \syn{\Gamma}_2\smcl\syn{\Delta}_2\mid \syn{a}:\syn{\alpha}
        [{\syn{S}_0/\syn{\Gamma}_0}\smcl{\syn{T}_0/\syn{\Delta}_0}]
        [{\syn{S}_1/\syn{\Gamma}_1}\smcl{\syn{T}_1/\syn{\Delta}_1}]\\
        \qquad\vdash
        \repl_{\syn{S}_0[\syn{S}_1],\syn{S}_0'[\syn{S}_1]\smcl\syn{T}_0[\syn{T}_1],\syn{T}_0'[\syn{T}_1]}\{\resti\{\syn{a}\}\}
        \equiv
        \resti\left\{\repl_{\syn{S}_0,\syn{S}_0'\smcl\syn{T}_0,\syn{T}_0'}\{\syn{a}\}
        [\syn{S}_1/\syn{\Gamma}_1\smcl\syn{T}_1/\syn{\Delta}_1]\right\}:\syn{\alpha}
        \left[\left.\syn{S}_0'[\syn{S}_1/\syn{\Gamma}_1]\right/\syn{\Gamma}_0\smcl
        \left.\syn{T}_0'[\syn{T}_1/\syn{\Delta}_1]\right/\syn{\Delta}_0\right]
        \end{array}}}
        \and   
        \inferrule*
        {{\syn{\Gamma}_1}\vdash \syn{S}_0/\syn{\Gamma}_0\\
        {\syn{\Delta}_1}\vdash \syn{T}_0/\syn{\Delta}_0\\
        \syn{\Gamma}_2\vdash \syn{S}_1\,/\,\syn{\Gamma}_1 \equiv \syn{S}_1'/\syn{\Gamma}_1\\
        \syn{\Delta}_2\vdash \syn{T}_1\,/\,\syn{\Delta}_1 \equiv \syn{T}_1'/\syn{\Delta}_1\\
        }
        {
        {\begin{array}{l}
        \syn{\Gamma}_2\smcl\syn{\Delta}_2\mid \syn{a}:\syn{\alpha}
        [{\syn{S}_0/\syn{\Gamma}_0}\smcl{\syn{T}_0/\syn{\Delta}_0}]
        [{\syn{S}_1/\syn{\Gamma}_1}\smcl{\syn{T}_1/\syn{\Delta}_1}]\\
        \qquad\vdash
        \repl_{\syn{S}_0[\syn{S}_1],\syn{S}_0[\syn{S}_1']\smcl\syn{T}_0[\syn{T}_1],\syn{T}_0[\syn{T}_1']}
        \{\resti\{\syn{a}\}\}
        \equiv
        \resti\left\{\repl_{\syn{S}_1,\syn{S}_1'\smcl\syn{T}_1,\syn{T}_1'}\{\syn{a}\}\right\}
        :\syn{\alpha}
        \left[\left.\syn{S}_0[\syn{S}_1']\right/\syn{\Gamma}_0\smcl
        \left.\syn{T}_0[\syn{T}_1']\right/\syn{\Delta}_0\right]
        \end{array}}}
        \and    
        \inferrule*
        {\ol{\syn{\Gamma}}\mid \syn{a}_1:\syn{\alpha}_1\smcl\dots\smcl\syn{a}_m:\syn{\alpha}_m\vdash \syn{\mu}:\syn{\beta}}
        {\ol{\syn{\Gamma}'}\mid \syn{a}_1:\syn{\alpha}_1[\syn{\Gamma}_0/\syn{\Gamma}_0\smcl\syn{\Gamma}_1/\syn{\Gamma}_1]\smcl\dots\smcl
        \syn{a}_m:\syn{\alpha}_m[\syn{\Gamma}_{m-1}/\syn{\Gamma}_{m-1}\smcl\syn{\Gamma}_m/\syn{\Gamma}_m]\vdash
        \reste\left\{\syn{\mu}[\ol{\syn{\Gamma}}/\ol{\syn{\Gamma}}]\right\}\equiv
        \syn{\mu}\{\reste\{\syn{a}_1\}\smcl\dots\smcl\reste\{\syn{a}_m\}\}:\syn{\beta}}
        \and
        \inferrule*
        {\ol{\syn{\Gamma}}\mid \syn{a}_1:\syn{\alpha}_1\smcl\dots\smcl\syn{a}_m:\syn{\alpha}_m\vdash \syn{\mu}:\syn{\beta}\\
        \syn{\Gamma}'_i\vdash \syn{S}_i\,/\,\syn{\Gamma}_i \ (i=0,\dots,m)\\
        \syn{\Gamma}''_i\vdash \syn{S}_i'\,/\,\syn{\Gamma}_i' \ (i=0,\dots,m)}
        {
        {\begin{array}{l}    
        \ol{\syn{\Gamma}''}\mid
        \syn{a}_1:\syn{\alpha}_1[\syn{S}_0/\syn{\Gamma}_0\smcl\syn{S}_1/\syn{\Gamma}_1][\syn{S}_0'/\syn{\Gamma}_0'\smcl\syn{S}_1'/\syn{\Gamma}_1']
        \smcl\dots\smcl
        \syn{a}_m:\syn{\alpha}_m[\syn{S}_{m-1}/\syn{\Gamma}_{m-1}\smcl\syn{S}_m/\syn{\Gamma}_m][\syn{S}_{m-1}'/\syn{\Gamma}_{m-1}'\smcl\syn{S}_m'/\syn{\Gamma}_m']\\
        \qquad\vdash
        \resti\left\{\syn{\mu}[\ol{\syn{S}}/\ol{\syn{\Gamma}}][\ol{\syn{S}}'/\ol{\syn{\Gamma}}']\right\}
        \equiv
        \left(\syn{\mu}\left[\ol{\syn{S}_i[\syn{S}_i'/\syn{\Gamma}_i']/\syn{\Gamma}_i}\right]\right)
        \left\{\resti\{\syn{a}_1\}\smcl\dots\smcl\resti\{\syn{a}_m\}\right\}:\syn{\beta}
        \left[\syn{S}_0[\syn{S}_0'/\syn{\Gamma}_0']\smcl\syn{S}_1[\syn{S}_1'/\syn{\Gamma}_1']\right]
        \end{array}}
        }
        \and
        \inferrule*
        {\ol{\syn{\Gamma}}\mid \syn{a}_1:\syn{\alpha}_1\smcl\dots\smcl\syn{a}_m:\syn{\alpha}_m\vdash \syn{\mu}:\syn{\beta}\\
        \syn{\Gamma}'_i\vdash \syn{S}_i\,/\,\syn{\Gamma}_i\equiv\syn{T}_i\,/\,\syn{\Gamma}_i \ (i=0,\dots,m)}
        {
        {\begin{array}{l}
        \ol{\syn{\Gamma}'}\mid
        \syn{a}_1:\syn{\alpha}_1[\syn{S}_0/\syn{\Gamma}_0\smcl\syn{S}_1/\syn{\Gamma}_1]\smcl\dots\smcl
        \syn{a}_m:\syn{\alpha}_m[\syn{S}_{m-1}/\syn{\Gamma}_{m-1}\smcl\syn{S}_m/\syn{\Gamma}_m]\\
        \qquad\vdash
        \repl_{\syn{S}_0,\syn{T}_0\smcl\syn{S}_m,\syn{T}_m}\left\{\syn{\mu}[\ol{\syn{S}}/\ol{\syn{\Gamma}}]\right\}
        \equiv
        \syn{\mu}\left[\ol{\syn{T}}/\ol{\syn{\Gamma}}\right]
        \left\{\repl_{\syn{S}_0,\syn{T}_0\smcl\syn{S}_1,\syn{T}_1}\{\syn{a}_1\}\smcl
        \dots\smcl\repl_{\syn{S}_{m-1},\syn{T}_{m-1}\smcl\syn{S}_m,\syn{T}_m}\{\syn{a}_m\}\right\}:\syn{\beta}
        \left[\syn{T}_0\smcl\syn{T}_m\right]        
        \end{array}}
        }
    \end{mathparpagebreakable}
