# Supplementary material for: An Internal Logic of Virtual Double Categories
Source: arXiv:2410.06792 source file (2025-01-23)
Supplement: Supplementary file 2 [file proofsynvdc.tex]

Justification of the derivation rules of an internal language has two parts:
to verify that each step of derivation is valid (soundness) and
to ensure that they are sufficient to derive all they should (completeness),
both with respect to the semantics.
In this paper, we have achived these two parts implicitly along the way,
but not thoroughly in the main text.
This is because theese sorts of verification always require massive effort of induction,
and it is not always easy to present them in a readable manner.
For \ac{FVDblTT} and its semantics in \acp{CFVDC},
all we need to justify the rules is the following:
\begin{enumerate}
    \labeleditem \label{prfsyn:1} The interpretation of typing judgments in \ac{FVDblTT}$^\crude$ is well-defined,
    and two (pro)terms that are derivably equal in \ac{FVDblTT}$^\crude$ are interpreted as equal in \acp{CFVDC}. \label{item:sound1}
    \labeleditem \label{prfsyn:2} When two (pro)terms are derivably equal in \ac{FVDblTT},
    so are their crude translations in \ac{FVDblTT}$^\crude$.
    For a derivable protype isomorphism judgment in \ac{FVDblTT},
    there is a corresponding pair of mutually inverse proterms in \ac{FVDblTT}$^\crude$,
    and they are interpreted as the same loose isomorphism in \acp{CFVDC}.
    \labeleditem \label{prfsyn:3} The syntactic \ac{VDC} $\dbl{S}^\crude(\Sigma,\zero{E})$ (\Cref{def:synvdccrude}) of a crude specification is indeed a \ac{CFVDC}.
    \labeleditem \label{prfsyn:4} When two (pro)terms are derivably equal in \ac{FVDblTT}$^\crude$,
    so are their decrude translations in \ac{FVDblTT}.
\end{enumerate}
Since \ac{FVDblTT}$^\crude$ connects \ac{FVDblTT} and \acp{CFVDC},
the two parts of the justification are split into the four points above.
We have footnoted where these ingredients are used implicitly in the main text.
We do not provide the full proof,
but instead illustrate the idea of the proof with instances.

\Cref{prfsyn:2,prfsyn:4} are straightforward to verify,
because the translations and the rules are defined in a way that they satisfy these properties.

What is critical to verify \Cref{prfsyn:1} concerns the interpretation of proterms and their equalities.
Once you define the interpretation of protypes,
at which point you choose restrictions of loose arrows and other data using some universal properties,
two derivably equal proterms involving protypes whose interpretations require these choices
are interpreted as equal in \acp{CFVDC} when you fix the choices.
For example, consider the following rule:
\[
    \scriptsize
    \inferrule*
    {\syn{\Gamma}_{i,j}\vdash\syn{S}_{i,j}\,/\,\syn{\Delta}_{i,j} \ (i=1,\dots,m,\ j=1,\dots,n_i)\\
    \ol{\syn{\Delta}_{i,\ul{j}}}\mid \syn{A}_i \vdash \syn{\mu}_i:\syn{\beta}_i \ (i=1,\dots,m) \\
    \wt{\syn{\Delta}_{\ul{i},\wt{j}}} \mid\syn{b}_1:\syn{\beta}_1\smcl\dots\smcl\syn{b}_n:\syn{\beta}_n \vdash\syn{\nu}: \syn{\gamma}}
    {\syn{\ol{\Gamma}}\mid \ol{\syn{A}}[\ol{\syn{S}}/\ol{\syn{\Delta}}]\vdash
    \syn{\nu}\{\ol{\syn{\mu}}/\ol{\syn{b}}\}[\ol{\syn{S}}/\ol{\syn{\Delta}}]\equiv
    \syn{\nu}\left[\ol{\wt{\syn{S}}}/\ol{\wt{\syn{\Delta}}}\right]\left\{\left.\ol{\syn{\mu}_{\ul{i}}[\ol{\syn{S}_{i,\ul{j}}}/\ol{\syn{\Delta}_{i,\ul{j}}}]}\right/
    \ol{\syn{b}_{\ul{i}}}\right\}:
    \syn{\gamma}[\syn{S}_{0,0}/\syn{\Delta}_{0,0}\smcl\syn{S}_{m,n_m}/\syn{\Delta}_{m,n_m}]}
\]
The interpretations of the proterms are shown to be equal using the universal properties of restriction and the following equalities
(here we omit the symbol $\sem{\cdot}$ for simplicity and the names of the cells are written in red):
\begin{align*}
    &\quad
    \begin{tikzcd}[ampersand replacement=\&, column sep=16ex, virtual]
        \syn{\Gamma}_{0,0}
        \sar[rrr, dashed, "{\ol{\syn{A}}[\ol{\syn{S}}/\ol{\syn{\Delta}}]}"]
        \ar[d, equal]
        \ar[drrr, phantom, "{\color{red}\syn{\nu}\{\ol{\syn{\mu}}/\ol{\syn{b}}\}[\ol{\syn{S}}/\ol{\syn{\Delta}}]}"]
        \&\&\&
        {\syn{\Gamma}_{m,n_m}}
        \ar[d, equal]
        \\
        \syn{\Gamma}_{0,0}
        \sar[rrr, dashed, "{\syn{\gamma}[\syn{S}_{0,0}/\syn{\Delta}_{0,0}\smcl\syn{S}_{m,n_m}/\syn{\Delta}_{m,n_m}]}"']
        \ar[d, "{\syn{S}_{0,0}}"']
        \ar[phantom, drrr, "{\color{red}\rest}"{below}]
        \&\&\&
        {\syn{\Gamma}_{m,n_m}}
        \ar[d, "{\syn{S}_{m,n_m}}"]
        \\
        \syn{\Delta}_{0,0}
        \sar[rrr, "{\syn{\gamma}}"']
        \&\&\&
        {\syn{\Delta}_{m,n_m}}
    \end{tikzcd}
    \\
    &\overset{(1)}{=}
    \begin{tikzcd}[ampersand replacement=\&, column sep=6ex, virtual]
        \syn{\Gamma}_{0,0}
        \ar[d, "{\syn{S}_{0,0}}"']
        \sar[r, "{\syn{\alpha}_{1,1}[\syn{S}_{0,1}/\syn{\Delta}_{0,1}\smcl\syn{S}_{1,0}/\syn{\Delta}_{1,0}]}"{above=1ex}]
        \ar[dr, phantom, "{\color{red}\rest}"]
        \&
        \syn{\Gamma}_{0,1}
        \ar[d, "{\syn{S}_{0,1}}"']
        \sar[rr,dashed]
        \ar[drr, phantom, "{\color{red}\ol\rest}"]
        \&\&
        \syn{\Gamma}_{1,0}
        \ar[d, "{\syn{S}_{1,0}}"']
        \sar[dashed,rrr]
        \ar[drrr, phantom, "{\color{red}\ol\rest}"]
        \&\&\&
        \syn{\Gamma}_{m,n_m}
        \ar[d, "{\syn{S}_{m,n_m}}"]
        \\
        \syn{\Delta}_{0,0}
        \sar[r, "{\syn{\alpha}_{1,1}}"']
        \ar[d, equal]
        \ar[drrr, phantom, "{\color{red}\syn{\mu}_1}"]
        \&
        \syn{\Delta}_{0,1}
        \sar[dashed,rr]
        \&\&
        \syn{\Delta}_{1,0}
        \sar[dashed,rrr]
        \ar[d, equal]
        \ar[drrr, phantom, "\cdots"]
        \&\&\&
        \syn{\Delta}_{m,n_m}
        \ar[d, equal]
        \\
        \syn{\Delta}_{0,0}
        \sar[rrr, "{\syn{\beta}_1}"']
        \ar[d,equal]
        \ar[drrrrrr, phantom, "{\color{red}\syn{\nu}}"]
        \&\&\&
        \syn{\Delta}_{1,0}
        \sar[rrr, dashed]
        \&\&\&
        \syn{\Delta}_{m,n_m}
        \ar[d,equal]
        \\
        \syn{\Delta}_{0,0}
        \sar[rrrrrr, "{\syn{\gamma}}"']
        \&\&\&\&\&\&
        \syn{\Delta}_{m,n_m}
    \end{tikzcd}
    \\
    &\overset{(2)}{=}
    \begin{tikzcd}[ampersand replacement=\&, column sep=6ex, virtual]
        \syn{\Gamma}_{0,0}
        \ar[d, equal]
        \sar[r, "{\syn{\alpha}_{1,1}[\syn{S}_{0,1}/\syn{\Delta}_{0,1}\smcl\syn{S}_{1,0}/\syn{\Delta}_{1,0}]}"{above=1ex}]
        \ar[drrr, phantom, "{\color{red}{\syn{\mu}_{1}[\ol{\syn{S}_{1,\ul{j}}}/\ol{\syn{\Delta}_{1,\ul{j}}}]}}"']
        \&
        \syn{\Gamma}_{0,1}
        \sar[rr,dashed]
        \&\&
        \syn{\Gamma}_{1,0}
        \ar[d, equal]
        \sar[dashed,rrr]
        \ar[drrr, phantom, "{\color{red}\cdots}"]
        \&\&\&
        \syn{\Gamma}_{m,n_m}
        \ar[d, equal]
        \\
        \syn{\Gamma}_{0,0}
        \sar[rrr, "{\syn{\beta}_1[\syn{S}_{0,0}/\syn{\Delta}_{0,0}\smcl\syn{S}_{1,0}/\syn{\Delta}_{1,0}]}"']
        \ar[d, "{\syn{S}_{0,0}}"']
        \ar[drrr, phantom, "{\color{red}\rest}"{below}]
        \&
        \&\&
        \syn{\Gamma}_{1,0}
        \sar[dashed,rrr]
        \ar[d, "{\syn{S}_{1,0}}"']
        \ar[drrr, phantom, "{\color{red}\ol\rest}"]
        \&\&\&
        \syn{\Gamma}_{m,n_m}
        \ar[d, "{\syn{S}_{m,n_m}}"]
        \\
        \syn{\Delta}_{0,0}
        \sar[rrr, "{\syn{\beta}_1}"']
        \ar[d,equal]
        \ar[drrrrrr, phantom, "{\color{red}\syn{\nu}}"]
        \&\&\&
        \syn{\Delta}_{1,0}
        \sar[rrr, dashed]
        \&\&\&
        \syn{\Delta}_{m,n_m}
        \ar[d,equal]
        \\
        \syn{\Delta}_{0,0}
        \sar[rrrrrr, "{\syn{\gamma}}"']
        \&\&\&\&\&\&
        \syn{\Delta}_{m,n_m}
    \end{tikzcd}
    \\
    &\overset{(3)}{=}
    \begin{tikzcd}[ampersand replacement=\&, column sep=6ex, virtual]
        \syn{\Gamma}_{0,0}
        \ar[d, equal]
        \sar[r, "{\syn{\alpha}_{1,1}[\syn{S}_{0,1}/\syn{\Delta}_{0,1}\smcl\syn{S}_{1,0}/\syn{\Delta}_{1,0}]}"{above=1ex}]
        \ar[drrr, phantom, "{\color{red}{\syn{\mu}_{1}[\ol{\syn{S}_{1,\ul{j}}}/\ol{\syn{\Delta}_{1,\ul{j}}}]}}"]
        \&
        \syn{\Gamma}_{0,1}
        \sar[rr,dashed]
        \&\&
        \syn{\Gamma}_{1,0}
        \ar[d, equal]
        \sar[dashed,rrr]
        \ar[drrr, phantom, "{\color{red}\cdots}"]
        \&\&\&
        \syn{\Gamma}_{m,n_m}
        \ar[d, equal]
        \\
        \syn{\Gamma}_{0,0}
        \sar[rrr,]
        \ar[d, equal]
        \ar[drrrrrr, phantom, "{\color{red}\syn{\nu}[\ol{\wt{\syn{S}}}/\ol{\wt{\syn{\Delta}}}]}"]
        \&
        \&\&
        \syn{\Gamma}_{1,0}
        \sar[dashed,rrr]
        \&\&\&
        \syn{\Gamma}_{m,n_m}
        \ar[d, equal]
        \\
        \syn{\Gamma}_{0,0}
        \sar[rrrrrr, dashed, "{\syn{\gamma}[\syn{S}_{0,0}/\syn{\Delta}_{0,0}\smcl\syn{S}_{m,n_m}/\syn{\Delta}_{m,n_m}]}"']
        \ar[d, "{\syn{S}_{0,0}}"']
        \ar[phantom, drrrrrr, "{\color{red}\rest}"{below}]
        \&\&\&\&\&\&
        {\syn{\Gamma}_{m,n_m}}
        \ar[d, "{\syn{S}_{m,n_m}}"]
        \\
        \syn{\Delta}_{0,0}
        \sar[rrrrrr, "{\syn{\gamma}}"']
        \&\&\&\&\&\&
        {\syn{\Delta}_{m,n_m}}
    \end{tikzcd}
    \\
    &\overset{(4)}{=}
    \begin{tikzcd}[ampersand replacement=\&, column sep=16ex, virtual]
        \syn{\Gamma}_{0,0}
        \sar[rrr, dashed, "{\ol{\syn{A}}[\ol{\syn{S}}/\ol{\syn{\Delta}}]}"]
        \ar[d, equal]
        \ar[drrr, phantom, "{\color{red}\syn{\nu}\left[\ol{\wt{\syn{S}}}/\ol{\wt{\syn{\Delta}}}\right]\left\{\left.\ol{\syn{\mu}_{\ul{i}}[\ol{\syn{S}_{i,\ul{j}}}/\ol{\syn{\Delta}_{i,\ul{j}}}]}\right/
        \ol{\syn{b}_{\ul{i}}}\right\}}"]
        \&\&\&
        {\syn{\Gamma}_{m,n_m}}
        \ar[d, equal]
        \\
        \syn{\Gamma}_{0,0}
        \sar[rrr, dashed, "{\syn{\gamma}[\syn{S}_{0,0}/\syn{\Delta}_{0,0}\smcl\syn{S}_{m,n_m}/\syn{\Delta}_{m,n_m}]}"']
        \ar[d, "{\syn{S}_{0,0}}"']
        \ar[phantom, drrr, "{\color{red}\rest}"{below}]
        \&\&\&
        {\syn{\Gamma}_{m,n_m}}
        \ar[d, "{\syn{S}_{m,n_m}}"]
        \\
        \syn{\Delta}_{0,0}
        \sar[rrr, "{\syn{\gamma}}"']
        \&\&\&
        {\syn{\Delta}_{m,n_m}}
    \end{tikzcd}
\end{align*}
$\ol\rest$ represents the horizontal concatenation of restrictions cells.
The definition of the interpretation of substitutions $\left[\,\ol{-}/\ol{-}\,\right]$ are used in the equalities (1), (2), and (3),
and the definition of the interpretation of prosubstitutions $\{-/-\}$ is used in the equalities (1) and (4).
Because of the universal properties of restriction,
we can show that the interpretations of the two proterms are equal.

\Cref{prfsyn:3} is presented as \Cref{prop:crudevdc} in the main text,
and is the most nontrivial part of the four.
We give a more detailed explanation of the proof of \Cref{prfsyn:3} here.
Let us recall the definition of the syntactic \ac{VDC} $\dbl{S}^\crude(\Sigma,\zero{E})$ (\Cref{def:synvdccrude}).
In this virtual double category, 
a cell 
\begin{equation*}
    \begin{tikzcd}[column sep=8ex,virtual]
        {\syn{\Gamma}_0}
        \sar[r, "{\syn{\alpha}_1}"]
        \ar[d, "{\syn{S}_0}"']
        \ar[phantom,rrrd, "{\syn{\mu}}" description]
        &
        \cdots
        &
        \cdots
        \sar[r, "{\syn{\alpha}_n}"]
        &
        {\syn{\Gamma}_n}
        \ar[d,"\syn{S}_1"]
        \\
        {\syn{\Delta}_0}
        \sar[rrr, "{\syn{\beta}}"'] 
        &
        &&
        {\syn{\Delta}_1}
    \end{tikzcd}
\end{equation*}
is an equivalence class of proterms
\[
\syn{\ol{\Gamma}}\mid \syn{a}_1:\syn{\alpha}_1\smcl\dots\smcl\syn{a}_n:\syn{\alpha}_n
\vdash \syn{\mu}:\syn{\beta}[\syn{S}_0/\syn{\Delta}_0\smcl\syn{S}_n/\syn{\Delta}_n]
\]
modulo equality judgments derivable from $(\Sigma,\zero{E})$.
The identity cell on $\syn{\alpha}$ is given by the equivalence class of the provariable $\syn{\alpha}$ as a proterm.
A general composition of cells 
\[
    \begin{tikzcd}[column sep=4em,virtual]
        \syn{\Gamma}_{0,0}
        \ar[d, "\syn{S}_0"']
        \sard[r, "{\ol{\syn{\alpha}_1}}"]
        \ar[dr, phantom, "\syn{\mu}_1"]
        & \syn{\Gamma}_{1,0}
        \ar[d, "\syn{S}_1"']
        \sard[r, "\ol{\syn{\alpha}_{2}}"]
        \ar[dr, phantom, "\syn{\mu}_2"]
        & \syn{\Gamma}_{2,0}
        \ar[d, "\syn{S}_2"']
        \sard[r]
        & \cdots
        \sard[r, "\ol{\syn{\alpha}_m}"]
        \ar[dr, phantom, "\syn{\mu}_m"]
        & \syn{\Gamma}_{m,0}
        \ar[d, "\syn{S}_n"] \\
        \syn{\Delta}_{0}
        \ar[d, "\syn{T}_0"']
        \sar[r, "\syn{\beta}_1"']
        \ar[drrrr, phantom, "\syn{\nu}"]
        & \syn{\Delta}_{1}
        \sar[r, "\syn{\beta}_2"']
        & \syn{\Delta}_{2}
        \sar[r]
        & \cdots
        \sar[r, "\syn{\beta}_m"']
        & \syn{\Delta}_{m} 
        \ar[d, "\syn{T}_1"] \\
        \syn{\Theta}_{0}
        \sar[rrrr, "\syn{\gamma}"']
        & & & & \syn{\Theta}_{1}
    \end{tikzcd}
\]
is given as follows:
first, the cells $\syn{\mu}_i$'s and $\syn{\nu}$ are 

{\scriptsize
\begin{align*}
    \ol{\syn{\Gamma}_{i-1,\ul{j}}}&\mid \syn{a}_{i,1}:\syn{\alpha}_{i,1}\smcl\dots\smcl\syn{a}_{i,n_i}:\syn{\alpha}_{i,n_i}
    \vdash \syn{\mu}_i:\syn{\beta}_i[\syn{S}_{i-1}/\syn{\Delta}_{i-1}\smcl\syn{S}_{i}/\syn{\Delta}_{i}],
    & (i=1,\dots,m)\\
    \ol{\syn{\Delta}_{\ul{i}}}&\mid \syn{b}_1:\syn{\beta}_1\smcl\dots\smcl\syn{b}_m:\syn{\beta}_m
    \vdash \syn{\nu}:\syn{\gamma}[\syn{T}_0/\syn{\Theta}_0\smcl\syn{T}_1/\syn{\Theta}_1].
\end{align*}
}
From the second proterm, we can derive the proterm
{
\scriptsize
\[
    \wt{\syn{\Gamma}_{\ul{i},\wt{j}}}\mid
    \syn{b}_1:\syn{\beta}_1[\syn{S}_{0}/\syn{\Delta}_{0}\smcl\syn{S}_{1}/\syn{\Delta}_{1}]\smcl\dots\smcl
    \syn{b}_m:\syn{\beta}_m[\syn{S}_{0}/\syn{\Delta}_{0}\smcl\syn{S}_{1}/\syn{\Delta}_{1}]
    \vdash \resti\fow\left\{\syn{\nu}\left[\ol{\syn{S}}/\ol{\syn{\Delta}}\right]\right\}:\syn{\gamma}\left[\syn{T}_0[\syn{S}_0/\syn{\Delta}_0]\smcl\syn{T}_1[\syn{S}_1/\syn{\Delta}_1]\right].
\]
}

The proof of \Cref{prfsyn:3} is to show that this gives a well-defined \ac{CFVDC}.
Once we have shown it is a \ac{VDC},
the rest of the proof is routine as explained in the main text.
The laws for the identities follow from the first two axioms in \Cref{sec:appendix0}.
The hardest part of the proof is to show that the composition of cells is associative.
The proof is as follows:
the associativity of the composition of cells is presented as

{\tiny
    \[
    \left(\lambda\{\nu_1\smcl\dots\smcl\nu_m\}\right)\{\mu_{1,1}\smcl\dots\smcl\mu_{1,n_1}\smcl\dots\smcl\mu_{m,1}\smcl\dots\smcl\mu_{m,n_m}\}
    =
    \lambda\left\{\nu_1\{\mu_{1,1}\smcl\dots\smcl\mu_{1,n_1}\}\smcl\dots\smcl\nu_m\{\mu_{m,1}\smcl\dots\smcl\mu_{m,n_m}\}\right\}
    \]
}
for any cells $\lambda,\nu_1,\dots,\nu_m,\mu_{i,j}$ which are appropriately composable.
For the syntactic \ac{VDC}, this amounts to showing that,
for any proterms $\syn{\lambda},\syn{\nu}_1,\dots,\syn{\nu}_m,\syn{\mu}_{i,j}$ as follows:

{
\tiny          
    \begin{align*}
        \ol{\syn{\Theta}}\mid \ol{\syn{c}_{\ul{i}}}:\ol{\syn{\gamma}_{\ul{i}}} &\vdash \syn{\lambda}: \syn{\delta}[\syn{U}_0/\syn{\Phi}_0\smcl\syn{U}_1/\syn{\Phi}_1],\\ 
        \ol{\syn{\Delta}_{i-1,\ul{j}}}\mid \ol{\syn{b}_{i,\ul{j}}}:\ol{\syn{\beta}_{i,\ul{j}}} &\vdash 
        \syn{\nu}_i: \syn{\gamma}_i[\syn{T}_{i-1}/\syn{\Theta}_{i-1}\smcl\syn{T}_i/\syn{\Theta}_i], & (i=1,\dots,m)\\
        \ol{\syn{\Gamma}_{i-1,j-1,\ul{k}}}\mid \ol{\syn{a}_{i,j,\ul{k}}}:\ol{\syn{\alpha}_{i,j,\ul{k}}} &\vdash
        \syn{\mu}_{i,j}: \syn{\beta}_{i,j}[\syn{S}_{i-1,j-1}/\syn{\Delta}_{i-1,j-1}\smcl\syn{S}_{i-1,j}/\syn{\Delta}_{i-1,j}],
        & (i=1,\dots,m,\ j=1,\dots,n_i)
    \end{align*}
}
the following equality is derivable:
{
\tiny
\begin{align*}
    &
    \left(\resti\fow\left\{
    \left(\left(\resti\fow\left\{\syn{\lambda}\left[\ol{\syn{T}_{\ul{i}}}/\ol{\syn{\Theta}_{\ul{i}}}\right]
    \right\}\right)\left\{\ol{\syn{\nu}_{\ul{i}}}/\ol{\syn{c}_{\ul{i}}}\right\}\right)
    \left[\ol{\syn{S}_{\ul{i,j}}}/\ol{\syn{\Delta}_{\ul{i,j}}}\right]\right\}\right)
    \left\{\ol{\syn{\mu}_{\ul{i,j}}}/\ol{\syn{b}_{\ul{i,j}}}\right\}
    \\
    &\equiv
    \left(\resti\fow\left\{\syn{\lambda}\left[\left.\rol{\syn{T}_{\rul{i}}[\bol{\syn{S}_{\rul{i},\bul{j}}}/\bol{\syn{\Delta}_{\rul{i},\bul{j}}}]}\right/\rol{\syn{\Theta}_{\rul{i}}}
    \right]\right\}\right)
    \left\{\left.\rol{
    \left(\resti\fow\left\{\syn{\nu}_i\left[\bol{\syn{S}_{\rul{i}-1,\bul{j}}}/\bol{\syn{\Delta}_{\rul{i}-1,\bul{j}}}\right]\right\}\right)
    \left\{\bol{\syn{\mu}_{\rul{i},\bul{j}}}/\bol{\syn{b}_{\rul{i},\bul{j}}}\right\}}\right/
    \rol{\syn{c}_{\rul{i}}}\right\}
\end{align*}.
}
This is proved as follows: ({\tiny$\wt{\wt{\syn{S}}}/\wt{\wt{\syn{\Delta}}}=\syn{S}_{0,0}/\syn{\Delta}_{0,0}\smcl\syn{S}_{m,n_m}/\syn{\Delta}_{m,n_m}$})
{\tiny
\begin{align*}
    (\text{LHS})&\equiv
    \left(\resti\fow
    \left\{
    \left(
    \resti\fow
    \left\{\syn{\lambda}
    \left[\rol{\syn{T}_{\rul{i}}}/\rol{\syn{\Theta}_{\rul{i}}}\right]
    \left\{\rol{\syn{\nu}_{\rul{i}}}/\rol{\syn{c}_{\rul{i}}}\right\}
    \right\}
    \right)
    \left[\gol{\syn{S}_{\gul{i,j}}}/\gol{\syn{\Delta}_{\gul{i,j}}}\right]
    \right\}
    \right)
    \left\{\gol{\syn{\mu}_{\gul{i,j}}}/\gol{\syn{b}_{\gul{i,j}}}\right\}
    \\
    &\equiv %%%%% 1
    \left(\resti\fow
    \left\{
    \left(
    \resti\fow
    \left\{\syn{d}
    \right\}
    \left\{        
    \left. 
    \syn{\lambda}
    \left[\rol{\syn{T}_{\rul{i}}}/\rol{\syn{\Theta}_{\rul{i}}}\right]
    \left\{\rol{\syn{\nu}_{\rul{i}}}/\rol{\syn{c}_{\rul{i}}}\right\}
    \right/\syn{d}
    \right\}
    \right)
    \left[\gol{\syn{S}_{\gul{i,j}}}/\gol{\syn{\Delta}_{\gul{i,j}}}\right]
    \right\}
    \right)
    \left\{\gol{\syn{\mu}_{\gul{i,j}}}/\gol{\syn{b}_{\gul{i,j}}}\right\}
    \\
    &\equiv %%%%% 2
    \left(\resti\fow
    \left\{
    \left(
    \resti\fow
    \left\{\syn{d}
    \right\}
    \left[\wt{\wt{\syn{S}}}/\wt{\wt{\syn{\Delta}}}\right]
    \right)
    \left\{        
    \left. 
    \syn{\lambda}
    \left[\rol{\syn{T}_{\rul{i}}}/\rol{\syn{\Theta}_{\rul{i}}}\right]
    \left\{\rol{\syn{\nu}_{\rul{i}}}/\rol{\syn{c}_{\rul{i}}}\right\}
    \left[\gol{\syn{S}_{\gul{i,j}}}/\gol{\syn{\Delta}_{\gul{i,j}}}\right]
    \right/\syn{d}
    \right\}
    \right\}
    \right)
    \left\{\gol{\syn{\mu}_{\gul{i,j}}}/\gol{\syn{b}_{\gul{i,j}}}\right\}
    \\
    &\equiv %%%%% 3
    \left(\resti\fow
    \left\{
    \resti\fow
    \left\{\syn{d}\right\}
    \left[\wt{\wt{\syn{S}}}/\wt{\wt{\syn{\Delta}}}\right]
    \right\}\right)
    \left\{        
    \left. 
    \syn{\lambda}
    \left[\rol{\syn{T}_{\rul{i}}}/\rol{\syn{\Theta}_{\rul{i}}}\right]
    \left\{\rol{\syn{\nu}_{\rul{i}}}/\rol{\syn{c}_{\rul{i}}}\right\}
    \left[\gol{\syn{S}_{\gul{i,j}}}/\gol{\syn{\Delta}_{\gul{i,j}}}\right]
    \right/
    \syn{d}
    \right\}
    \left\{\gol{\syn{\mu}_{\gul{i,j}}}/\gol{\syn{b}_{\gul{i,j}}}\right\}
    \\
    &\equiv %%%%% 4
    \left(\resti\fow
    \left\{
    \resti\fow
    \left\{
    \syn{\lambda}
    \left[\rol{\syn{T}_{\rul{i}}}/\rol{\syn{\Theta}_{\rul{i}}}\right]
    \left\{\rol{\syn{\nu}_{\rul{i}}}/\rol{\syn{c}_{\rul{i}}}\right\}
    \left[\gol{\syn{S}_{\gul{i,j}}}/\gol{\syn{\Delta}_{\gul{i,j}}}\right]
    \right\}
    \right\}\right)
    \left\{\gol{\syn{\mu}_{\gul{i,j}}}/\gol{\syn{b}_{\gul{i,j}}}\right\}
    \\
    &\equiv %%%%% 5
    \left(\resti\fow
    \left\{
    \resti\fow
    \left\{
    \left(
    \syn{\lambda}
    \left[\rol{\syn{T}_{\rul{i}}}/\rol{\syn{\Theta}_{\rul{i}}}\right]
    \left[\wt{\syn{S}_{\ul{i},\tilde{j}}}/\wt{\syn{\Delta}_{\ul{i},\tilde{j}}}\right]
    \right)
    \left\{
    \left.    
    \rol{\syn{\nu}_{\rul{i}}}
    \left[\bol{\syn{S}_{\rul{i}-1,\bul{j}}}/\bol{\syn{\Delta}_{\rul{i}-1,\bul{j}}}\right]
    \right/
    \rol{\syn{c}_{\rul{i}}}\right\}
    \right\}
    \right\}\right)
    \left\{\gol{\syn{\mu}_{\gul{i,j}}}/\gol{\syn{b}_{\gul{i,j}}}\right\}
    \\
    &\equiv %%%%% 6
    \left(\resti\fow
    \left\{
    \left(
    \resti\fow
    \left\{
    \syn{\lambda}
    \left[\rol{\syn{T}_{\rul{i}}}/\rol{\syn{\Theta}_{\rul{i}}}\right]
    \left[\wt{\syn{S}_{\ul{i},\tilde{j}}}/\wt{\syn{\Delta}_{\ul{i},\tilde{j}}}\right]
    \right\}
    \right)
    \left\{
    \left.    
    \rol{\syn{\nu}_{\rul{i}}}
    \left[\bol{\syn{S}_{\rul{i}-1,\bul{j}}}/\bol{\syn{\Delta}_{\rul{i}-1,\bul{j}}}\right]
    \right/
    \rol{\syn{c}_{\rul{i}}}\right\}
    \right\}\right)
    \left\{\gol{\syn{\mu}_{\gul{i,j}}}/\gol{\syn{b}_{\gul{i,j}}}\right\}
    \\
    &\equiv %%%%% 7
    \left(
    \resti\fow
    \left\{
    \left(
    \syn{\lambda}
    \left[
    \left.\rol{\syn{T}_{\rul{i}}[\bol{\syn{S}_{\rul{i},\bul{j}}}/\bol{\syn{\Delta}_{\rul{i},\bul{j}}}]}
    \right/\rol{\syn{\Theta}_{\rul{i}}}
    \right]
    \left\{
    \rol{\resti\fow}/\rol{\syn{c}_{\rul{i}}}
    \right\}
    \right)
    \left\{
    \left.    
    \rol{\syn{\nu}_{\rul{i}}}
    \left[\bol{\syn{S}_{\rul{i}-1,\bul{j}}}/\bol{\syn{\Delta}_{\rul{i}-1,\bul{j}}}\right]
    \right/
    \rol{\syn{c}_{\rul{i}}}\right\}
    \right\}\right)
    \left\{\gol{\syn{\mu}_{\gul{i,j}}}/\gol{\syn{b}_{\gul{i,j}}}\right\}
    \\
    &\equiv %%%%% 8
    \left(
    \resti\fow
    \left\{
    \syn{\lambda}
    \left[
    \left.\rol{\syn{T}_{\rul{i}}[\bol{\syn{S}_{\rul{i},\bul{j}}}/\bol{\syn{\Delta}_{\rul{i},\bul{j}}}]}
    \right/\rol{\syn{\Theta}_{\rul{i}}}
    \right]
    \left\{
    \left.
    \rol{\resti\fow\left\{\syn{\nu}_{\rul{i}}\left[\bol{\syn{S}_{\rul{i}-1,\bul{j}}}/\bol{\syn{\Delta}_{\rul{i}-1,\bul{j}}}\right]\right\}}
    \right/\rol{\syn{c}_{\rul{i}}}
    \right\}
    \right\}\right)
    \left\{\gol{\syn{\mu}_{\gul{i,j}}}/\gol{\syn{b}_{\gul{i,j}}}\right\}
    \\
    &\equiv %%%%% 9
    \left(
    \resti\fow
    \left\{
    \syn{\lambda}
    \left[
    \left.\rol{\syn{T}_{\rul{i}}[\bol{\syn{S}_{\rul{i},\bul{j}}}/\bol{\syn{\Delta}_{\rul{i},\bul{j}}}]}
    \right/\rol{\syn{\Theta}_{\rul{i}}}
    \right]\right\}\right)
    \left\{
    \left.
    \rol{\resti\fow\left\{\syn{\nu}_{\rul{i}}\left[\bol{\syn{S}_{\rul{i}-1,\bul{j}}}/\bol{\syn{\Delta}_{\rul{i}-1,\bul{j}}}\right]\right\}}
    \right/\rol{\syn{c}_{\rul{i}}}
    \right\}
    \left\{\gol{\syn{\mu}_{\gul{i,j}}}/\gol{\syn{b}_{\gul{i,j}}}\right\}
    \\
    &\equiv (\text{RHS}).
\end{align*}
}
